# Supplementary material for: Incentivized Learning in Principal-Agent Bandit Games
Source: arXiv:2403.03811 source file (2024-03-06)
Supplement: Supplementary file 1 [file technical.tex]

\section{Additional Technical Results}\label{app:technical}

\begin{lemma}\label{lemma:bounded_incentives}
    Assume that we run \Cref{algorithm:binary_search}. Then, for any $a \in \cA, t\in [T]$, $0 \leq \licv_a(t) \leq \icvmid_a(t) \leq \uicv_a(t)  \leq 1$.
\end{lemma}

\begin{proof}[Proof of \Cref{lemma:bounded_incentives}]
    We consider an action $a \in \cA$ and a number of binary searches $N \in \N$ run on this action. Suppose that we run an additional binary search round on action $a$ at some time $t$
    \begin{equation}
    \label{lemBIbound}
    \icvmid_a(N) = \frac{\uicv_a(N)+\licv_a(N)}{2} \Rightarrow \icvmid_a(N) \in [\licv_a(N), \uicv_a(N)] \eqsp.
    \end{equation}
    After this iteration of binary search, we have
    \begin{align}
    \label{equation:iteration_lemma_bounded_incentives}
        \uicv_a(N+1) &= \indi{a}(A_t)\icvmid_a(N) + (1-\indi{a}(A_t)) \uicv_a(N) \\
        \licv_a(N+1) &=  (1-\indi{a}(A_t))\icvmid_a(N) + \indi{a}(A_t)\licv_a(N) \eqsp.
    \end{align}
    \Cref{equation:iteration_lemma_bounded_incentives} together with \Cref{lemBIbound} gives
    \begin{align*}
    & \licv_a(N+1) \geq \licv_a(N) \\
    & \uicv_a(N+1) \leq \uicv_a(N) \eqsp.
    \end{align*}
    However, for any action $a\in \cA$, the binary search was initialized with $\licv_a(0) = 0$ and $\uicv_a(0) = 1$. Therefore a trivial induction shows that for any $N \in \N$, we have
    \begin{equation*}
    0 \leq \licv_a(N) \leq \icvmid_a(N) \leq \uicv_a(N) \leq 1 \eqsp.
    \end{equation*}
\end{proof}

\begin{lemma}\label{lemma:precision_incentives}
Assume that at some step $t\in [T]$, we have run $D(t)$ iterations of binary search on each action $a \in \cA$. Then for any action $a \in \cA$
\begin{equation*}
    \icvstar_a \in [\licv_a(D_t), \uicv_a(D_t)] \: \text{ and } \: |\uicv_a(D_t) - \licv_a(D_t) | \leq \frac{1}{2^{D(t)}} \eqsp.
\end{equation*}
\end{lemma}

\begin{proof}[Proof of \Cref{lemma:precision_incentives}]
Considering some arm $a$, we carry out an induction on the number of binary searches $D(t)$ that have been run on $a$. The initialisation holds since $\licv_a(0) = 0$ and $\uicv_a(0) = 1$. We suppose that the property is true for some $D(t) \in \N^\star$ and we run one more binary search on each arm.
\begin{equation*}
\icvmid_a(D(t)+1) = \frac{\uicv_a(D(t)) + \licv_a(D(t))}{2} \eqsp,
\end{equation*}
$\icvmid_a(D(t))$ being the incentive offered to the agent if he chooses action $a$. Depending on the action chosen by the agent, we have the following update
\begin{comment}
\begin{align*}
    &\1(A_{D(t)} = a) = \1(\icvmid_a(D(t)) \geq \icvstar_a) \\
    \Longleftrightarrow \; &\1(A_{D(t)} = a) = \1(\icvmid_a(D(t)) \geq \icvstar_a) \eqsp.
\end{align*}
\end{comment}
\begin{equation*}
    \1(\{A_{D(t)} = a\}) = \1(\{\icvmid_a(D(t)) \geq \icvstar_a\}) \eqsp.
\end{equation*}
Therefore
\begin{align*}
    \uicv_a(D(t)+1) & = \1(\{A_{D(t)} = a\})\icvmid_a(D(t)) + \1(\{A_{D(t)} \ne a\})\uicv_a(D(t)) \\
    \licv_a(D(t)+1) & = \1(\{A_{D(t)} \ne a\})\icvmid_a(D(t)) + \1(\{A_{D(t})= a\})\licv_a(D(t)) \eqsp.
\end{align*}
Consequently
\begin{align*}
    & \icvstar_a \in [\licv_a(D(t)+1), \uicv_a(D(t)+1)] \\
    \text{and: } & \uicv_a(D(t)+1) - \licv_a(D(t)+1) = \frac{\uicv_a(D(t)) - \licv_a(D(t))}{2} \eqsp.
\end{align*}
Since the binary search was initialized with $\licv_a(0) = 0$ and $\uicv_a(0) = 1$, a trivial induction gives for any $t, D(t)$
\begin{equation*}
    \uicv_a(D(t)) - \licv_a(D(t)) \leq \frac{1}{2^{D(t)}} \eqsp.
\end{equation*}
\end{proof}
